# Supplementary material for: Graph Deep Learning for Intracranial Aneurysm Blood Flow Simulation and Risk Assessment
Source: arXiv:2512.09013 source file (2025-12-09)
Supplement: Supplementary file 1 [file notation.tex]

\todo{todo}

\begin{table}[h!]
    \centering
    \begin{tabular}{l|l}
    \toprule
    \multicolumn{2}{c}{Simulation notation} \\ \midrule
    $\numnodes \in \mathbb{N}$ & Number of atoms in a crystal \\
    $\mat = (\coords, \types, \lattice)$ & A crystal structure \\
    $\coords \in [0, 1)^{3 \times \numnodes}$ & Fractional atomic coordinates \\
    $\cartcoords \in \mathbb{R}^{3 \times \numnodes}$ & Cartesian atomic coordinates \\
    $\types \in \mathbb{A}^\numnodes$ & Atomic species in a crystal \\
    $\lattice = (\lvec\nindex{1}, \lvec\nindex{2}, \lvec\nindex{3}) \in \mathbb{R}^{3\times3}$ & The unit cell lattice matrix \\
    $\lvec\nindex{j} \in \mathbb{R}^3$, $j \in \{1, 2, 3\}$ & The $j$-th lattice vector \\
    $\mV = (\vv_1, \vv_2, \ldots \vv_N) \in \mathbb{R}^{d \times N}$  & Concatenation of $N$ $d$-dimensional column vectors into a matrix \\
    $\edgeset \subset \{1, 2, \ldots, \numnodes\}^2 \times \mathbb{Z}^3 $ & Set of edges in a material \\
    $\nodesel, \othernodesel \in \{1, 2, \ldots, \numnodes\}$ & Index of an atom in a material \\
    $\hiddendim \in \mathbb{N}$ & The number of hidden dimension in our GNN\\
    $\bm{1}_n \in\mathbb{R}^{n}$ & $n$-dimensional column vector containing ones \\
    \bottomrule
    \multicolumn{2}{c}{Graph Neural Network notation} \\
    \midrule
    $\tdisc \in {1, 2, \ldots, T}$ & Diffusion timestep  \\
    $T \in \mathbb{N}$ & Number of time discretization steps for the diffusion process \\
    $q(\coord\tindex{0})$ & The data distribution \\
    $q(\coord\tindex{\tdisc} | \coord\tindex{\tdisc-1})$ & Single-step diffusion transition kernel \\
    $q(\coord\tindex{\tdisc} | \coord\tindex{0})$ & One-shot diffusion kernel \\
    $q(\coord\tindex{T})$ & Prior (noise) distribution \\
    $\vs_\vtheta(\cdot, \tdisc)$ & Score model \\
    $\vs_{\coords, \vtheta}(\cdot, \tdisc)$ & Score model for atomic coordinates\\
    $\log p_\vtheta(\types\tindex{0} | \coords\tindex{\tdisc}, \lattice\tindex{\tdisc}, \types\tindex{\tdisc}, \tdisc)$ & Predicted logits for atom types at $\tdisc=0$. \\
    $\vs_{\lattice, \vtheta}(\cdot, \tdisc)$ & Score model for lattice\\
    $\vz$ & Standard Gaussian noise $\vz \sim \mathcal{N}(\vzero, \mI)$ \\
    \bottomrule
    \end{tabular}
    \caption{Table of notations}
    \label{tab:notation_table}
\end{table}
