# Supplementary material for: Graph Deep Learning for Intracranial Aneurysm Blood Flow Simulation and Risk Assessment
Source: arXiv:2512.09013 source file (2025-12-09)
Supplement: Supplementary file 2 [file results.tex]

\subsection{AnXplore}

\begin{figure}[!ht]
  \centering
  \includegraphics[width=0.99\textwidth]{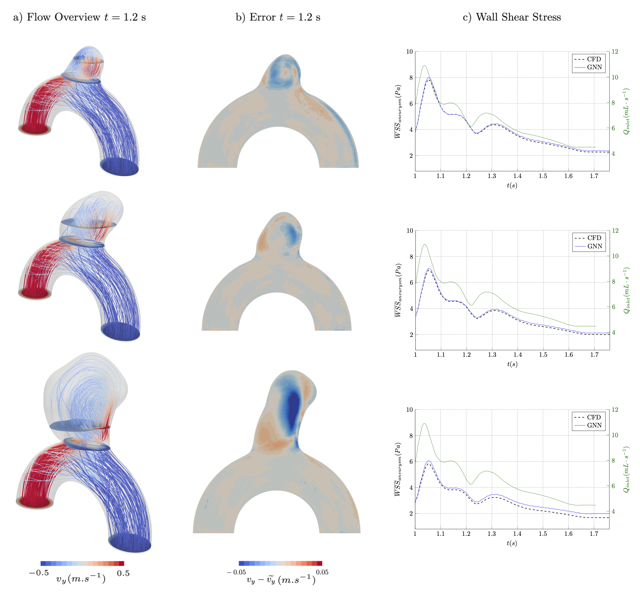}
  \caption{\small\textbf{Flow, errors and WSS for 3 meaningful samples from the test dataset. The same 3 samples are used in the following Figures \ref{fig:bulge_compar}, \ref{fig:rmse_osi}}
  \textbf{a)} Detailed flow analysis of the selected cases with Systolic flow lines. Legend presents $v_y$ in $mm/s$. We also highlight two plans: one at $y=8$ that we consider as the neck of the aneurysm, and one at $y=10$ that we consider as meaningful to represent the state of a trajectory. Those plans are reused in Figure \ref{fig:bulge_compar}.
  \textbf{b)} Magnitude of the error between the CFD and our model in the range $[0,500]$. The plan used is defined with the normal $\vec{n}=[0,1,0]$. We can see that most of the errors are present in the right part of the neck of the aneurysm, where the flow is the most difficult to simulate. 
  \textbf{c)} Comparison between the WSS from the CFD simulation and from our trajectory. Both trajectories yield very similar WSS. The parent vessel’s inflow rate is overlaid on all three graphs on the right for visualizing time shifts over the cardiac cycle.}
  \label{fig:flow_wss}
\end{figure}

\begin{figure}[!ht]
  \centering
  \includegraphics[width=0.99\textwidth]{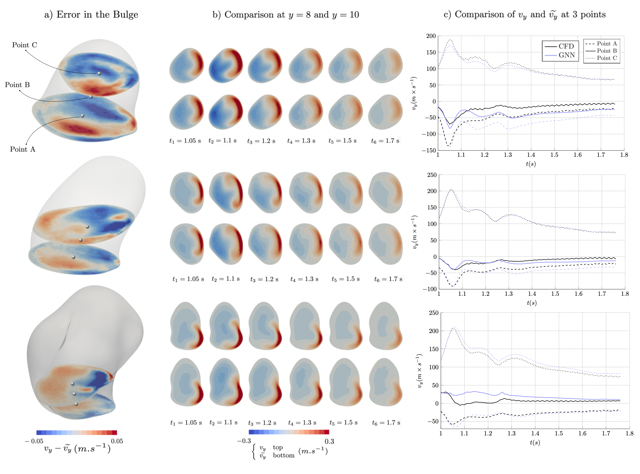}
  \caption{\small\textbf{Flow inside the aneurysm, 2D plan comparison and velocity comparison on three selected points.}
  \textbf{a)} Detailed flow analysis of the selected cases with Systolic flow lines inside of the bulge. The two highlighted plans are the same as before, at $y=8$ and $y=10$. The three selected points used in \textbf{c)} are showcased in green.
  \textbf{b)} Comparison between the CFD (top row) and our GNN (bottom row) for $v_y$ inside the bulge in a 2D plans defined by $x=0, y=10, z=0$. We can see the increase and decrease of velocity with the cardiac cycle, as well as a high fidelity trajectory from our method.
  \textbf{c)} Comparison on 3 selected points at $y=8, y=9, y=10$. Instability in the CFD solution is due to a discrepancy between the timestep used for our training and comparison ($\Delta t = 0.01$) and the one used to solve Navier-Stokes ($\Delta t = 0.002$). Differences in trajectories are within the range of differences between a rigid and an FSI simulation, showcasing how close to CFD our method is. (See Appendix X)}
  \label{fig:bulge_compar}
\end{figure}

\begin{figure}[!ht]
  \centering
  \includegraphics[width=0.99\textwidth]{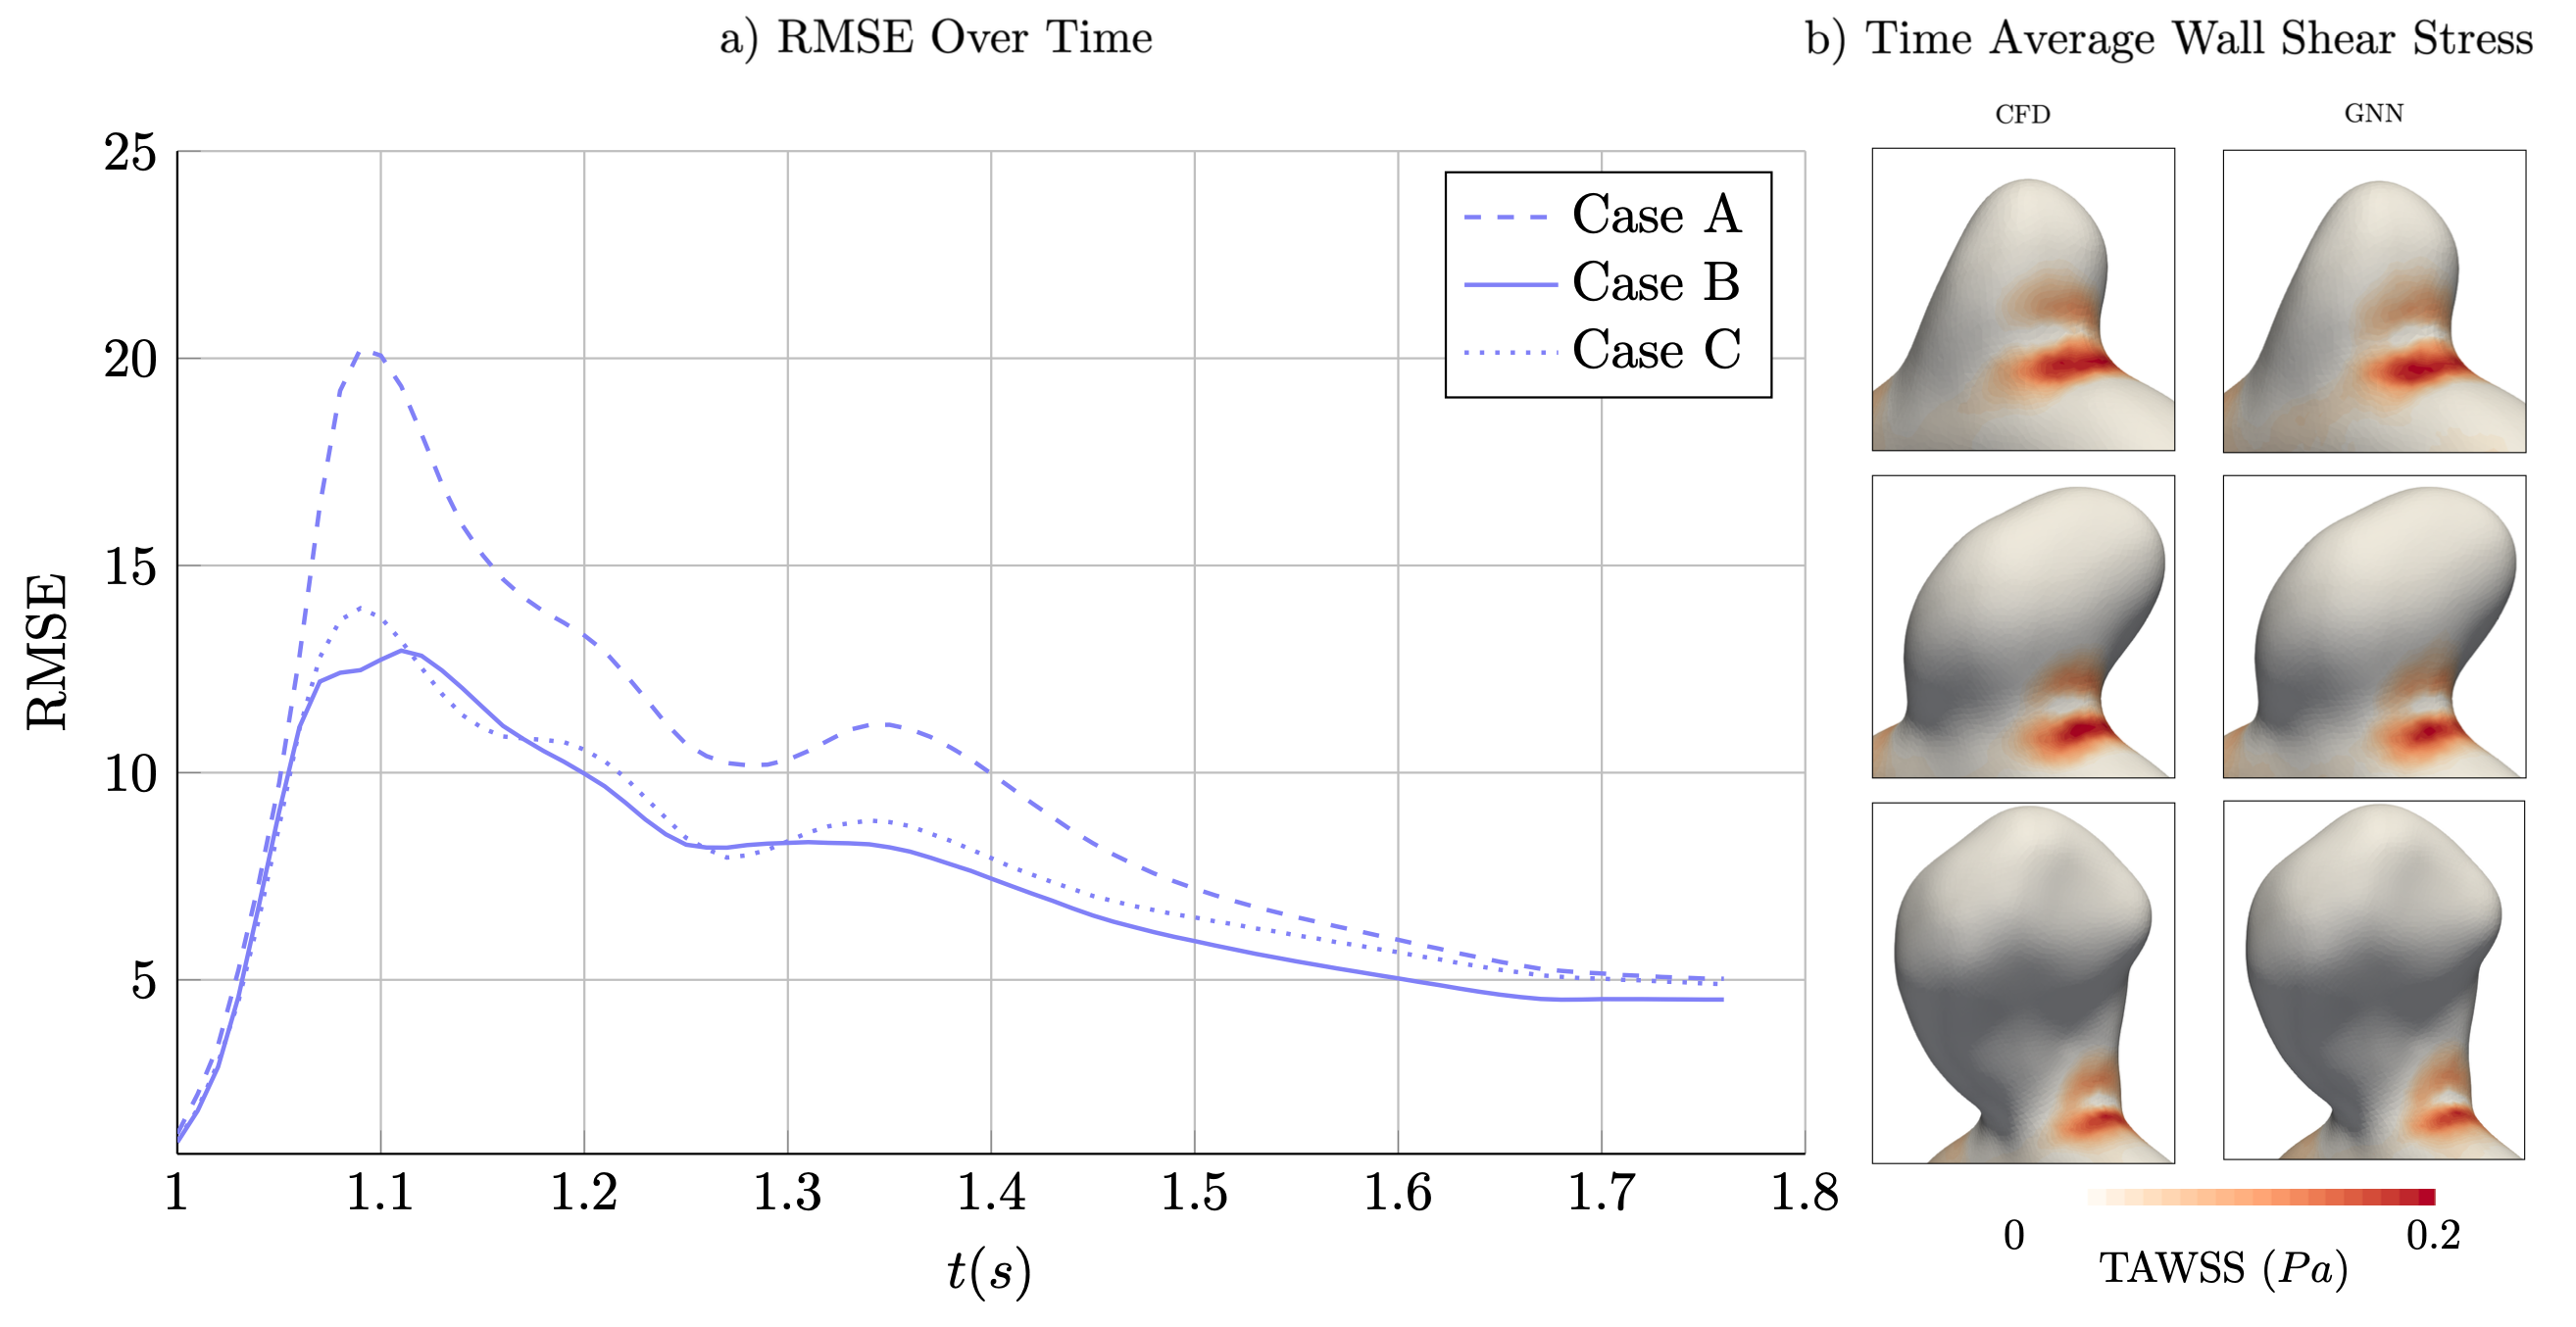}
  \caption{\small\textbf{RMSE overtime and comparison of Time Average WSS (TAWSS) and Oscillatory Shear Index (OSI) on the three selected aneurysms.}
  \textbf{a)} Root Mean Squared Error between the CFD and our method at each time step for the three aneurysms. A more detailed presentation of the error accross our dataset and its comparison between different methods is available in Appendix X.
  \textbf{b)} Comparison between the CFD (left) and our GNN (right) for the TAWSS around the bulge. Our method yields very similar results for this important metric for medical decisions.
  \textbf{c)}  Comparison between the CFD (left) and our GNN (right) for the OSI around the bulge. Our method does find the similar points of interests but also showcase a lot of noise inside the bulge.}
  \label{fig:rmse_osi}
\end{figure}

\subsection{MATCH}

\subsection{Physical quantities}

\subsubsection{Navier-Stokes Equation}

\subsubsection{Mass Conservation Equation}
