# Supplementary material for: Graph Deep Learning for Intracranial Aneurysm Blood Flow Simulation and Risk Assessment
Source: arXiv:2512.09013 source file (2025-12-09)
Supplement: Supplementary file 3 [file additional-results.tex]

\subsection{Comparison with other machine learning methods}

\subsection{Comparison with a Fluid-Structure Interaction solver}
